# Supplementary material for: DualOptim: Enhancing Efficacy and Stability in Machine Unlearning with Dual Optimizers
Source: arXiv:2504.15827 source file (2025-10-31)
Supplement: Supplementary file 1 [file algorithm.tex]

\section{Algorithm} \label{sec:alg}
\begin{algorithm}
\caption{Machine Unlearning with DualOptim}
\label{alg:dualoptim}
\begin{algorithmic}[1]
    \STATE {\bfseries Input:} Model: $f_\theta$; Forget set: $D_f=(\vx_f, \vy_f)$; Retain set: $D_r=(\vx_r, \vy_r)$; Iterations for outer loop: $T_{o}$; Iterations for forgetting: $T_f$; Iterations for retaining: $T_r$; Step size for forgetting: $\eta_f$; Step size for retaining: $\eta_r$
    \STATE $\mathrm{Optim}_f = \mathrm{Adam}(\theta, \eta_f)$\COMMENT{use Adam for forgetting}
    \STATE $\mathrm{Optim}_r = \mathrm{SGD}(\theta, \eta_r)$\COMMENT{use the default optimizer for retaining, e.g., SGD}
    \FOR{$t=1,...,T_{o}$}
        \FOR{$t'=1,...,T_{f}$}
        \STATE Fetch mini-batch data from forget set $B_f\sim D_f$
        \STATE Calculate the forget loss $\mathcal{L}_f$ on $B_f$ and get the gradient
        \STATE Use $\mathrm{Optim}_f$ to update $\theta$
        \ENDFOR
        \FOR{$t'=1,...,T_{r}$}
        \STATE Fetch mini-batch data from retain set $B_r\sim D_r$
        \STATE Calculate the retain loss $\mathcal{L}_r$ on $B_r$ and get the gradient
        \STATE Use $\mathrm{Optim}_r$ to update $\theta$
        \ENDFOR
    \ENDFOR
    \STATE {\bfseries Output:} Model $f_\theta$
\end{algorithmic}
\end{algorithm} 

The pseudo-code of DualOptim in machine unlearning (MU) is presented in Algorithm \ref{alg:dualoptim}. We integrate DualOptim in a general MU pipeline. In line 5-9, we first minimize the forget loss $\mathcal{L}_f$ using $\mathrm{Optim}_f$. In line 10-14, we minimize the retain loss $\mathcal{L}_r$ using $\mathrm{Optim}_r$. The model parameters $\theta$ are alternatively updated on $\mathcal{L}_f$ and $\mathcal{L}_r$. Note that $\mathcal{L}_f$ and $\mathcal{L}_r$ are dependent on different MU algorithms.
